# Supplementary material for: Simple and Efficient Hard Label Black-box Adversarial Attacks in Low Query Budget Regimes
Source: arXiv:2007.07210 source file (2021-06-11)
Supplement: Supplementary file 1 [file appendix.tex]

\begin{figure*}[t!]
\centering
\begin{subfigure}[b]{\textwidth}
   \includegraphics[width=\linewidth]{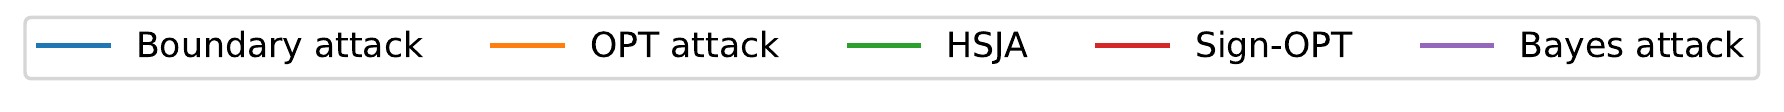}
\end{subfigure}

\begin{subfigure}[b]{0.32\textwidth}
   \includegraphics[width=1\linewidth]{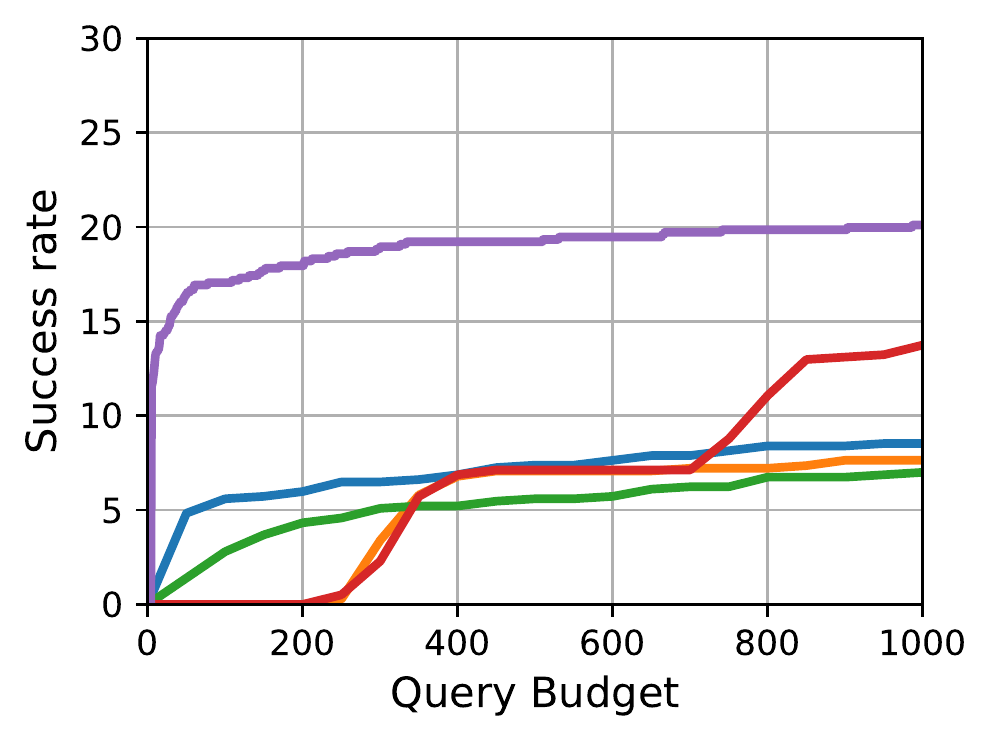}
   \caption{ {ResNet50}, $\epsilon=5.0$}
 
\end{subfigure}
\begin{subfigure}[b]{0.32\textwidth}
   \includegraphics[width=1\linewidth]{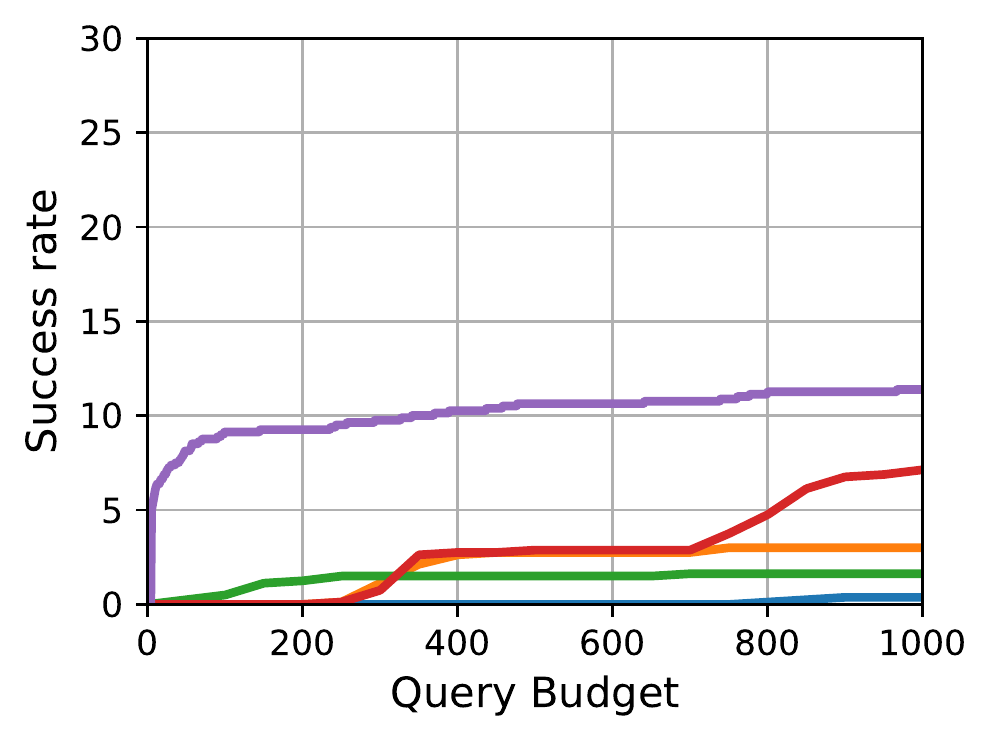}
   \caption{ {Inception-v3}, $\epsilon=5.0$}

\end{subfigure}
\begin{subfigure}[b]{0.32\textwidth}
   \includegraphics[width=1\linewidth]{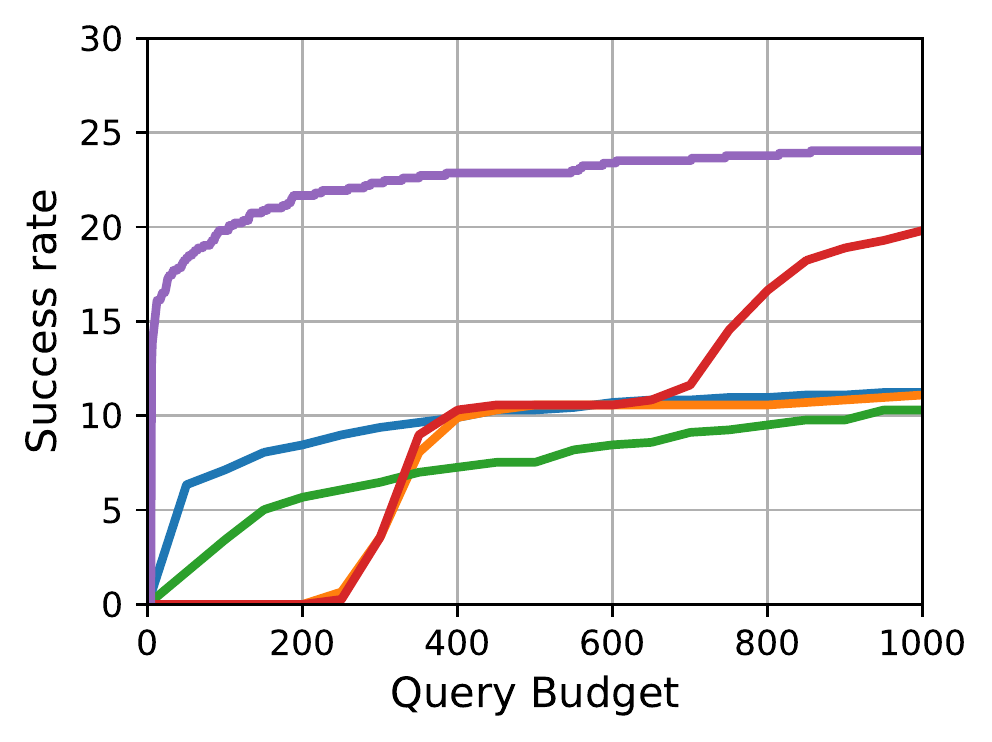}
   \caption{ {VGG16-bn}, $\epsilon=5.0$}

\end{subfigure}
\begin{subfigure}[b]{0.32\textwidth}
  \includegraphics[width=1\linewidth]{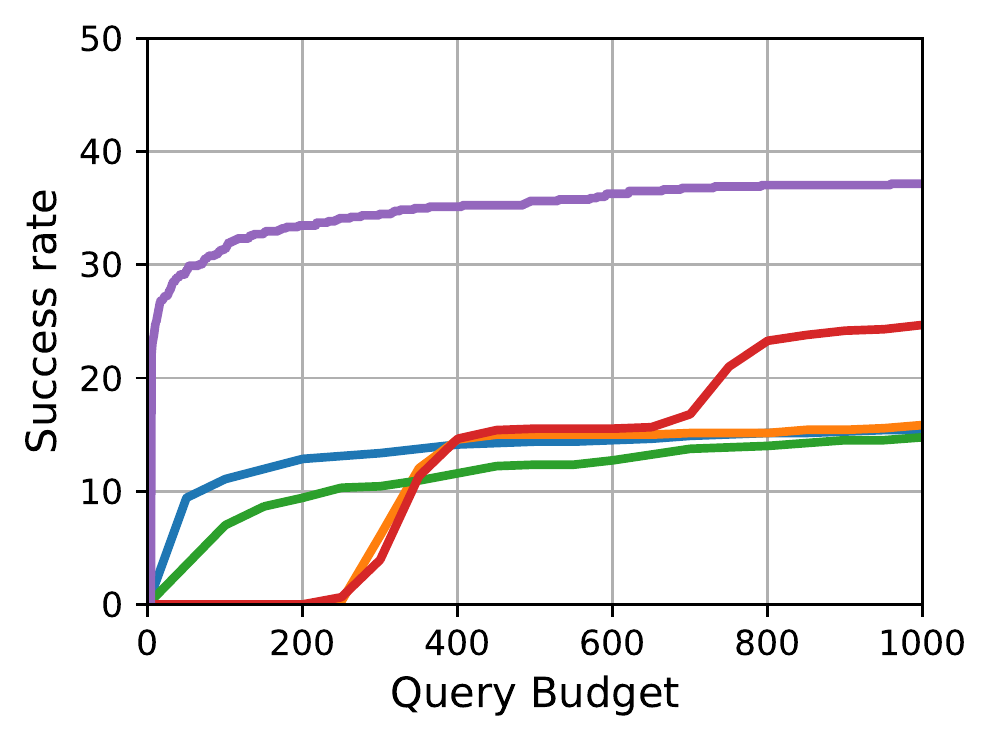}
  \caption{ {ResNet50}, $\epsilon=10.0$}

\end{subfigure}
\begin{subfigure}[b]{0.32\textwidth}
  \includegraphics[width=1\linewidth]{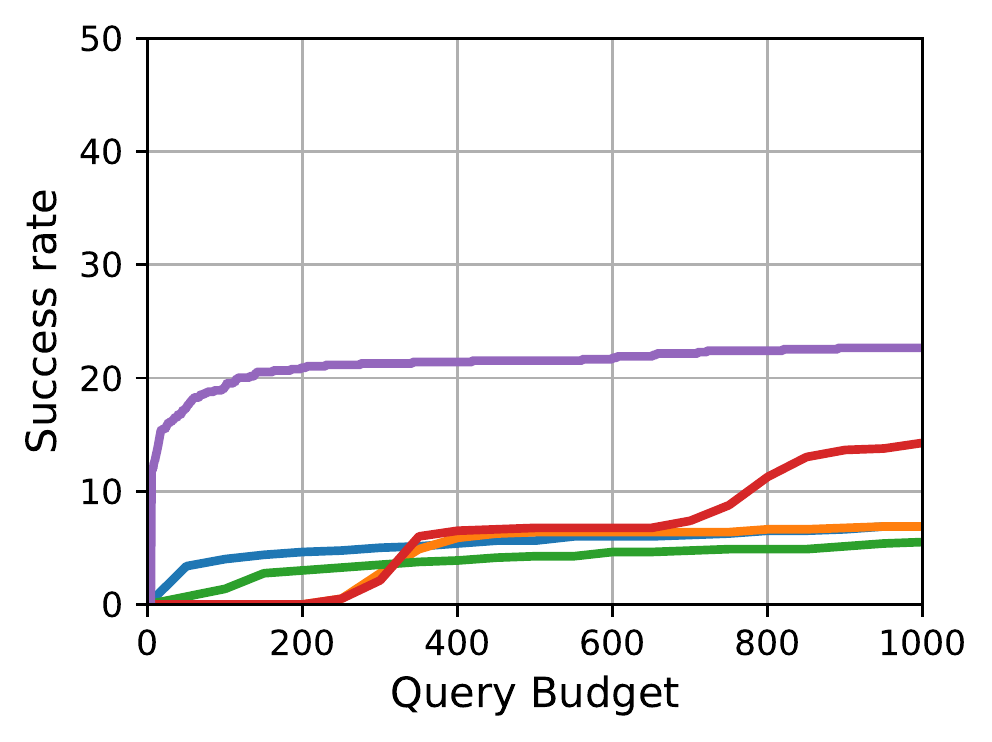}
  \caption{ {Inception-v3}, $\epsilon=10.0$}

\end{subfigure}
\begin{subfigure}[b]{0.32\textwidth}
  \includegraphics[width=1\linewidth]{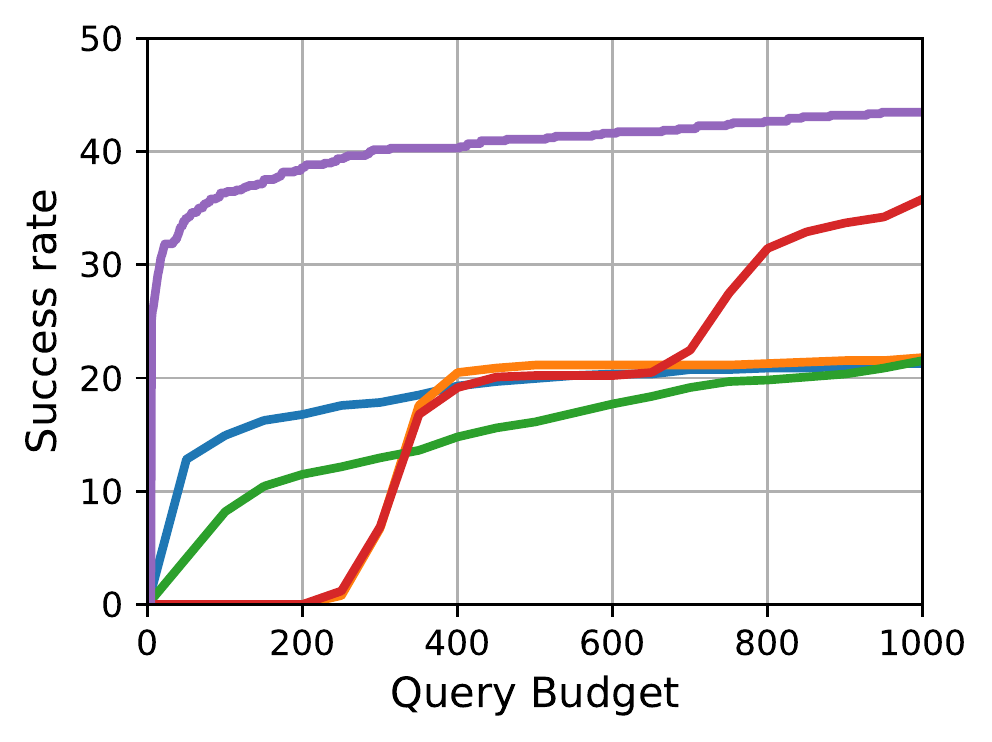}
  \caption{ {VGG16-bn}, $\epsilon=10.0$}
\end{subfigure}
\begin{subfigure}[b]{0.32\textwidth}
  \includegraphics[width=1\linewidth]{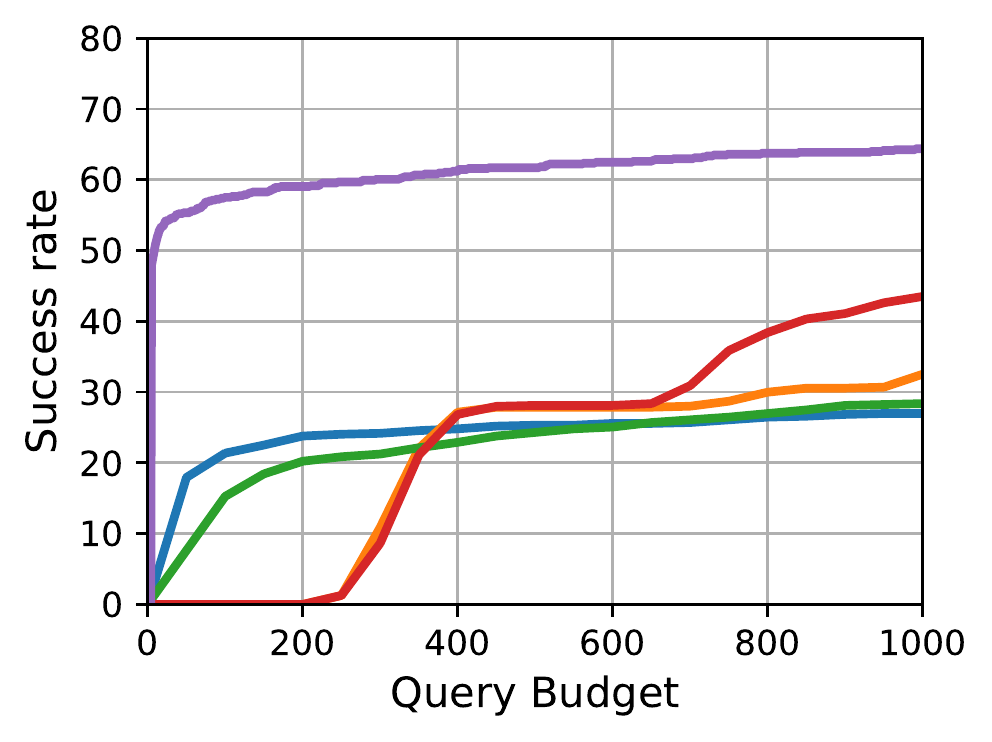}
  \caption{ {ResNet50}, $\epsilon=20.0$}

\end{subfigure}
\begin{subfigure}[b]{0.32\textwidth}
  \includegraphics[width=1\linewidth]{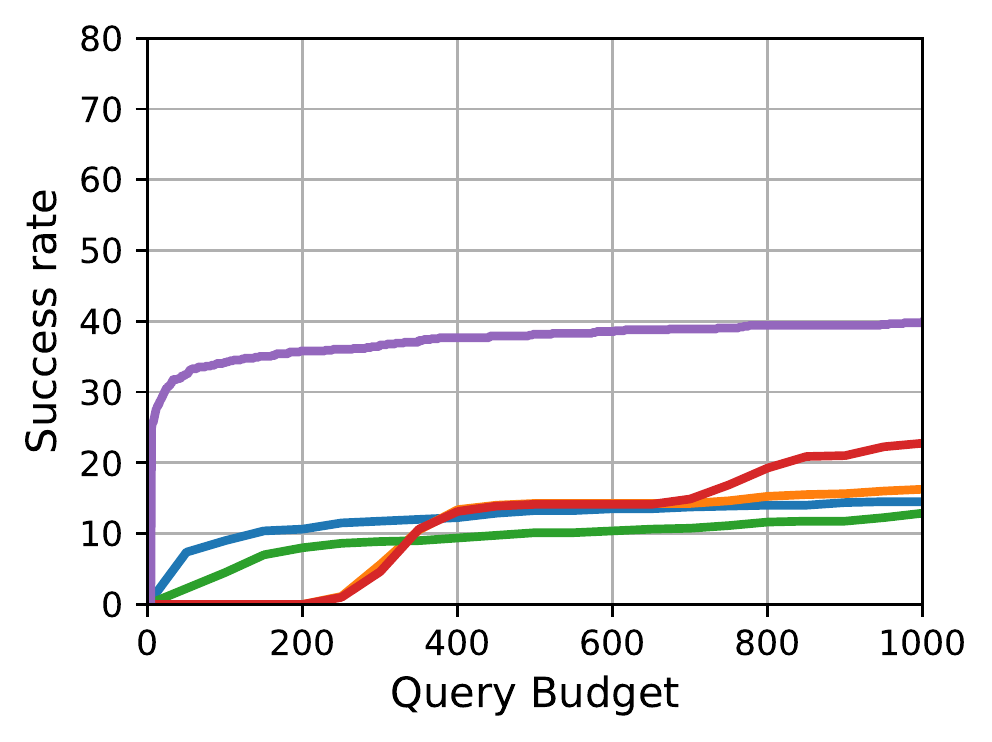}
  \caption{ {Inception-v3}, $\epsilon=20.0$}
\end{subfigure}
\begin{subfigure}[b]{0.32\textwidth}
  \includegraphics[width=1\linewidth]{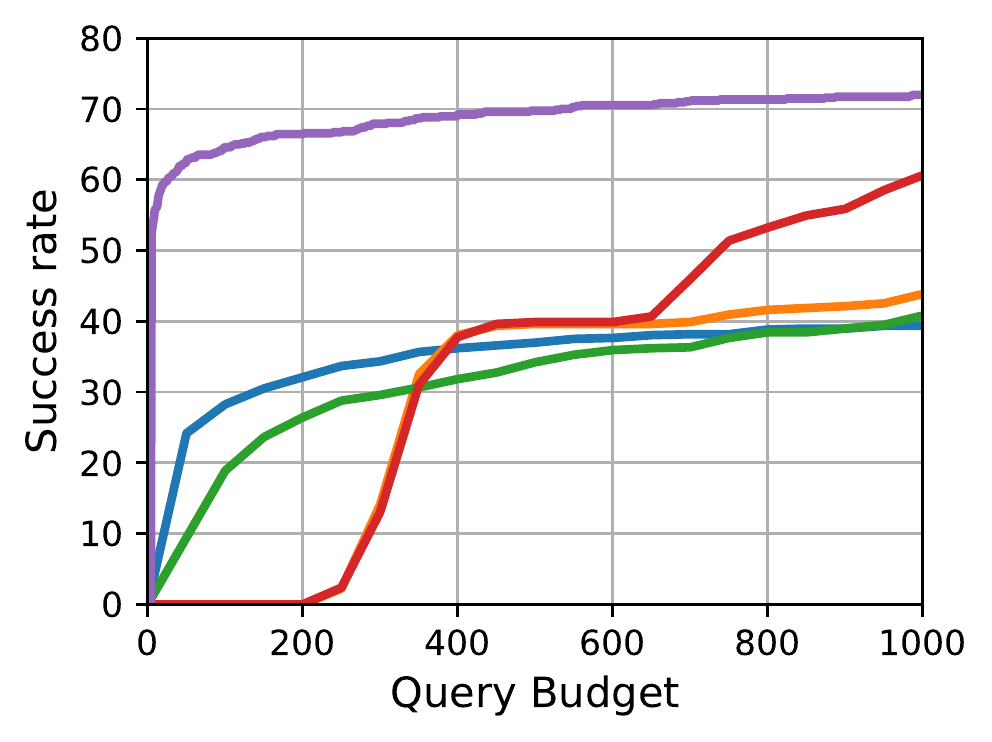}
  \caption{ {VGG16-bn}, $\epsilon=20.0$}
\end{subfigure}
\caption{Performance comparison for $\ell_2$ untargeted attacks on ImageNet classifiers for all methods and $\epsilon$ thresholds.}
\label{fig:pareto_l2_all}
\end{figure*}

\section{Additional Experiments and Results for Hard Label Black-box Attacks}

\subsection{Comparison under different query budgets}
Figure \ref{fig:pareto_l2_all} compares the performance of Bayes attack with that of baseline methods for $\ell_2$ untargeted attacks on all three ImageNet classifiers and three different $\epsilon$ thresholds for different query budgets. We can see that Bayes attack consistently outperforms the other baseline methods across all query budgets up to $1000$.

\subsection{Query Efficiency Comparison}
\begin{figure}[h!]
\centering
   \includegraphics[width=0.75\linewidth]{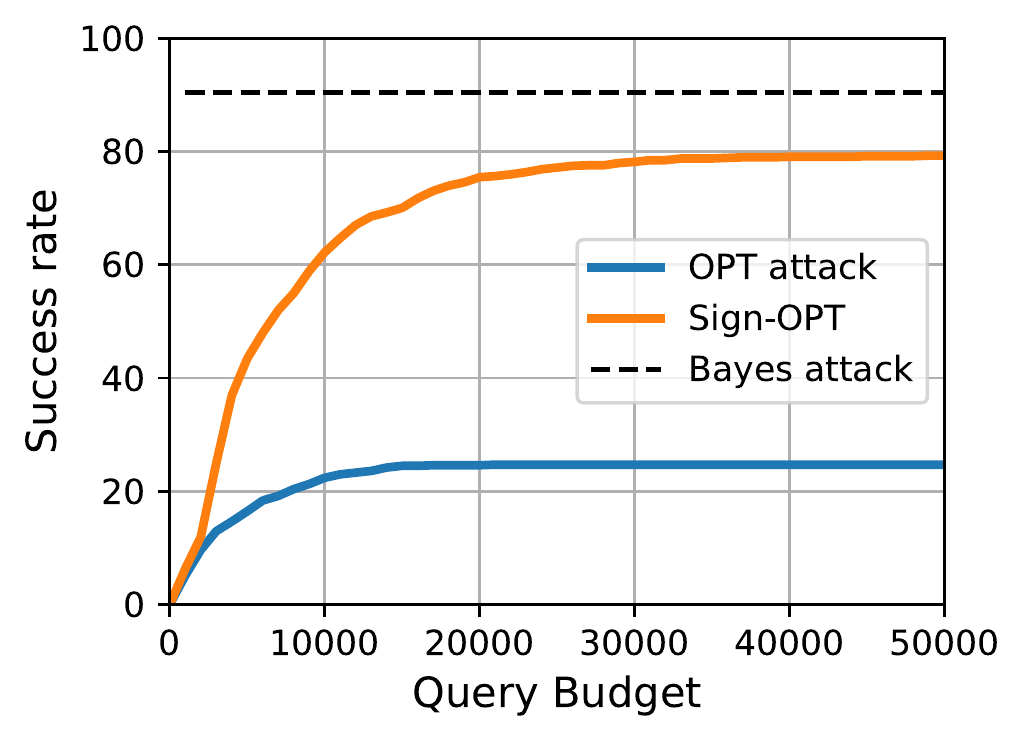}
   \caption{Performance comparison on MNIST.}
   \label{fig:pareto_mnist}
\end{figure}

\begin{figure}[h!]
\centering
   \includegraphics[width=0.75\linewidth]{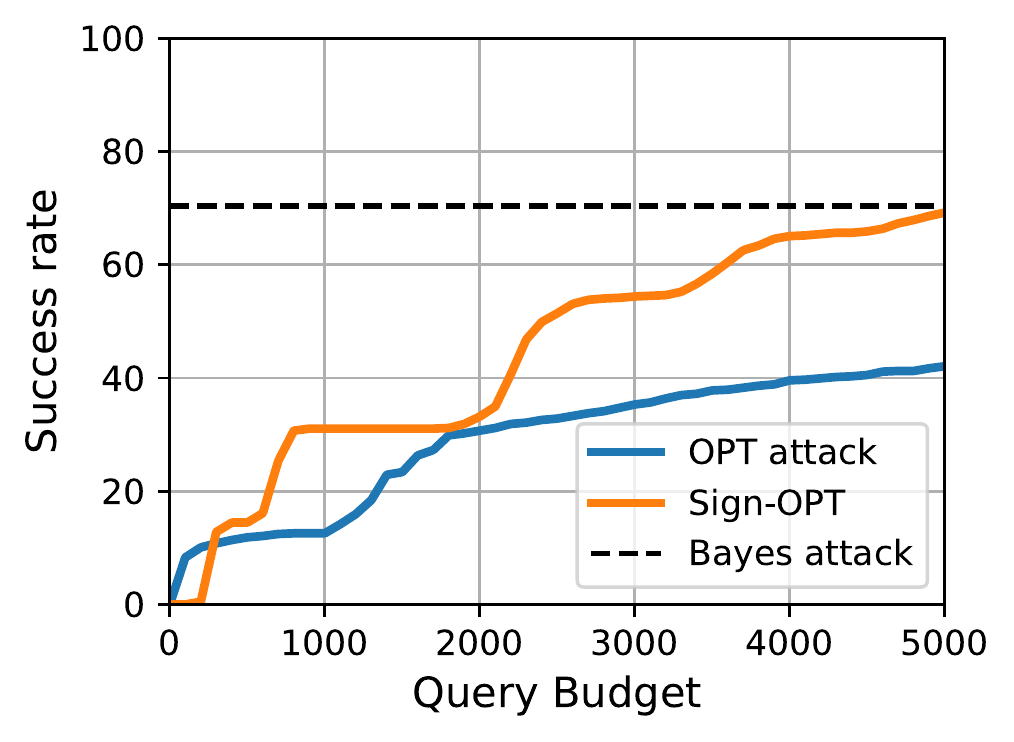}
   \caption{Performance comparison on CIFAR-10.}
   \label{fig:pareto_cifar}
\end{figure}

We compare the query efficiency of the competing methods on MNIST and CIFAR-10 for $\ell_\infty$ attacks. We run the competing methods until they achieve the same best attack success rate as Bayes attack or exceed a much higher query limit ($50000$ for MNIST and $5000$ for CIFAR-10). We use the same setting as described in Section 5.2. Figure \ref{fig:pareto_mnist} and \ref{fig:pareto_cifar} compare the performance on MNIST and CIFAR-10 respectively. For MNIST, we can see that even with $50 \times$ higher query budget than the Bayes attack, competing methods are not able to achieve similar attack success rate. For CIFAR-10, Sign-OPT requires $5 \times$ higher queries to achieve the same success rate as Bayes attack.

\subsection{Ablation Study}
In this section, we perform ablation studies on ImageNet by exploring different low dimensional structured subspaces and comparing mapping techniques for both $\ell_2$ and $\ell_\infty$ threat models. 

\subsubsection{Low Dimension Subspaces}
\label{sec:basis}
In case of the $\ell_2$ threat model, we utilize the low dimensional subspace generated by the low frequency sine and cosine FFT basis vectors. We can also consider the cosine FFT basis or sine FFT basis separately by using only the real components or imaginary components of the frequency domain representation. 
% Similarly, we can consider the sine FFT basis separately by considering the imaginary component of the frequency domain representation.

We compare the attacks generated in the low dimension subspace created using cosine and sine FFT basis vectors separately and together. For this experiment, we perform hard label black-box attacks on ResNet50 trained on ImageNet with $\ell_2$ perturbation set to 20.0. We maintain a query budget of 1000 across the experiments. For fair comparison, we keep the size of low dimension subspace almost same across the experiments, i.e. $3 \times 18 \times 18$ for cosine and sine FFT basis separately and $3 \times 12 \times 12 \times 2$ when considering the complete FFT basis. We also compare with a random set of vectors sampled from standard normal distribution. We keep the size of vectors sampled from normal distribution same as $3 \times 18 \times 18$.

 \begin{table}[ht]
\centering
\begin{tabular}{c c  c } 
 \toprule
 {\bf Basis } & {\bf Success} & {\bf Avg Queries} \\
 \midrule
 {Cosine FFT} & $  {64.38}	\% $ & $	{54.25}	 $ \\
 {Sine FFT}	    & $	{63.74}	\% $ & $	{45.72}	$ \\
 {Cosine and sine FFT} & $	{66.67}	\% $ & $	{54.97}	$\\
 {Standard Normal}  & $	{33.33}	\% $ & $	{48.25}	$ \\
 \bottomrule
 \end{tabular}
 \caption{Performance comparison of FFT basis vectors and random vectors sampled from the standard normal distribution for $\ell_2$ attack with $\epsilon=20.0$ on ResNet50.}
 \label{table:query_compare_fft}
 \end{table}
 
%  \begin{figure}[h]
% \centering
%   \includegraphics[width=0.7\linewidth]{icml_lowdim.pdf}
%   \caption{Comparison of FFT basis vectors and random vectors sampled from the standard normal distribution for $\ell_2$ attack with $\epsilon=20.0$ on ResNet50.}
% \label{fig:query_compare_fft}
% \end{figure}
 
 Table \ref{table:query_compare_fft} compares the performance of basis vectors in terms of attack success rate and average query count. We observe that the low frequency FFT basis vectors enhanced the attack accuracy significantly as compared to random set of vectors generated from standard normal distribution. On the other hand among low frequency components, sine and cosine FFT basis vectors together provide a slight gain in attack success rate as compared to using them separately. 
% Figure \ref{fig:query_compare_fft} shows the success rate at different query budgets.

\subsubsection{Mapping Techniques}
The proposed method requires a low dimensional subspace for efficiently searching the perturbation and a mapping technique for transforming the perturbation learnt in the low dimension to the full input space.  
We use FFT basis vectors for learning perturbation for $\ell_2$ threat model while nearest neighbor interpolation for $\ell_\infty$ threat model. Here, we compare both the methods on $\ell_2$ as well as $\ell_\infty$ threat models.

We compare both the mapping techniques on attacking ResNet50 trained on ImageNet with $\ell_\infty$ and $\ell_2$ perturbation set to $0.05$ and $20.0$, respectively. We maintain a query budget of 1000 across the experiments. For fair comparison, we keep the size of low dimension subspace same across the experiments, i.e. $3 \times 18 \times 18$. 

Table \ref{table:query_compare_upsampling} shows the performance of both the mapping techniques on $\ell_\infty$ and $\ell_2$ threat models. FFT basis vectors perform better than nearest neighbor interpolation in the $\ell_2$ threat model, while nearest neighbor performs better for $\ell_\infty$ threat model.

\begin{table}[h]
\centering
\begin{tabular}{c c  c c } 
 \toprule
{{ \bf Attack}} & {\bf Mapping } & {\bf Success} & {\bf Avg } \\
{\bf Type} & {\bf Technique} & {\bf Rate} &{\bf Queries}\\
 \midrule
\multirow{2}{*}{$\ell_\infty, \epsilon = 0.05$ } 
 
&	{IFFT} & $  {59.16}	\% $ & $	{55.72}	 $ \\
&	{NNI}	& $	{67.48}	\% $ & $	{45.94}	$ \\
\midrule
\multirow{2}{*}{$\ell_2, \epsilon = 20.0$}
&	{IFFT} & $	{66.67}	\% $ & $	{54.97}	 $ \\
&	{NNI}	& $	{59.54}	\% $ & $	{50.71} $  \\

 \bottomrule
 \end{tabular}
 \caption{Comparing inverse fast Fourier transform (IFFT) and nearest neighbor interpolation (NNI) for $\ell_2$ and $\ell_\infty$ attack on ResNet50.}
 \label{table:query_compare_upsampling}
 \end{table}
 
\section{Soft Label Black-box Attacks}
We also show results for soft label black-box adversarial attacks, where queries return the entire output layer of the network, either as logits or probabilities. The objective function for this setting is slightly different from the hard-label setting where queries to the network yield only the predicted class of the input, with no other information about the network’s final layer output.  We use an objective function suggested 
by \citet{carlini2017} and used in \citet{autozoom, zoo}:
\begin{align}
\label{eq:obj}
    &  \max_{\bm{\delta}} \, f(\mbf{x}, y, \bm{\delta}) \\
    & \text{subject to} \;\; \Vert \bm{\delta} \Vert_p \leq \epsilon \;\; \text{and} \;\;  (\mbf{x} + \bm{\delta}) \in [0, 1]^d, \nonumber \\
 \text{where } & f(\mbf{x}, y, \bm{\delta}) = \big\{\max_{k \neq y}\log[F(\mbf{x} + \bm{\delta})]_k - \log [F(\mbf{x} + \bm{\delta})]_{y} \big\} \nonumber
\end{align}
 The input $\mathbf{x} + \boldsymbol{\delta}$ to $f$ is an adversarial example for $F$ if and only if $f(\mathbf{x}, y, \boldsymbol{\delta}) > 0$.
 
\subsection{Experiments on ImageNet}
We compare the performance of  {Bayes attack} against three score-based black-box attacks $-$ {NES} \citep{nes}, {Bandits-TD} \citep{bandits} and {Parsimonious} \citep{parsimonious},  within the $\ell_\infty$ threat model. We evaluate the attack methods on the pretrained ResNet50, Inception-v3 and VGG16-bn for ImageNet. We use 10,000 randomly selected images (normalized to [0, 1]) from the ImageNet validation set that were initially correctly classified. We set the $\ell_\infty$ perturbation bound $\epsilon$ to $0.05$ and evaluate the performance of all the methods for low query budgets. 
For the baseline methods, we use the implementations made available  by  the  authors  and  use  hyperparameters  as  suggested in their respective papers.

\begin{figure*}[t]
\centering
\begin{subfigure}[b]{0.75\textwidth}
   \includegraphics[width=1\linewidth]{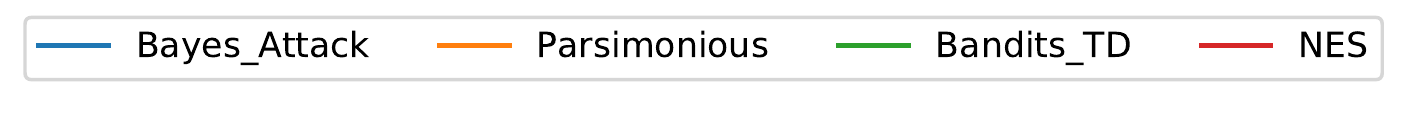}
\end{subfigure}

\begin{subfigure}[b]{0.32\textwidth}
   \includegraphics[width=1\linewidth]{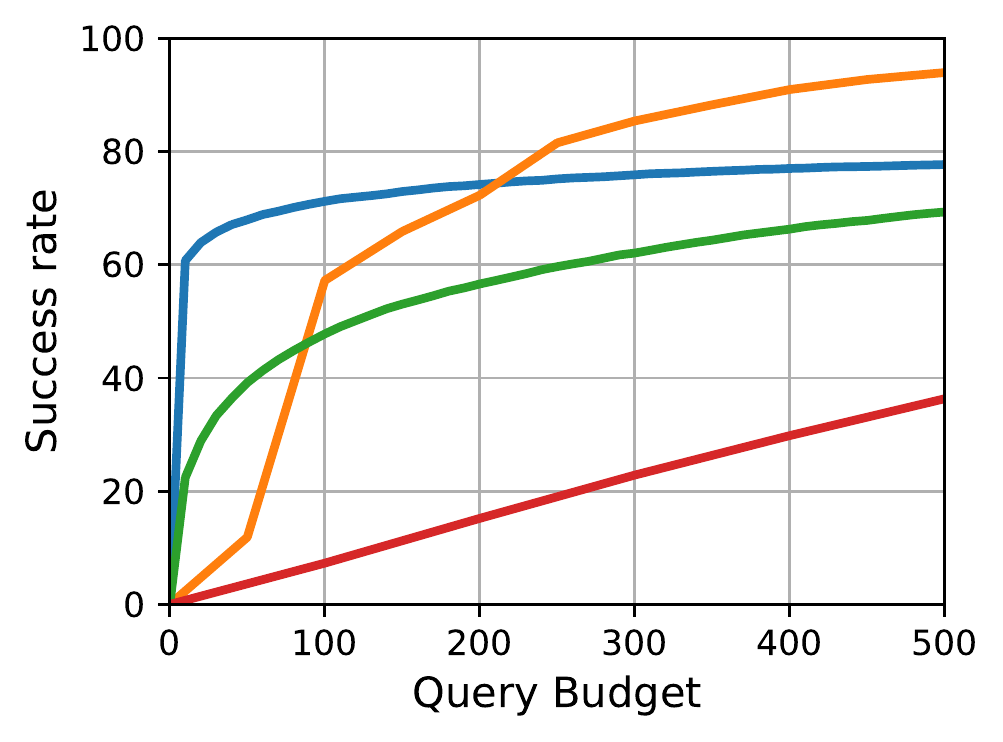}
   \caption{ {ResNet50}}
   \label{fig:resnet} 
\end{subfigure}
\begin{subfigure}[b]{0.32\textwidth}
   \includegraphics[width=1\linewidth]{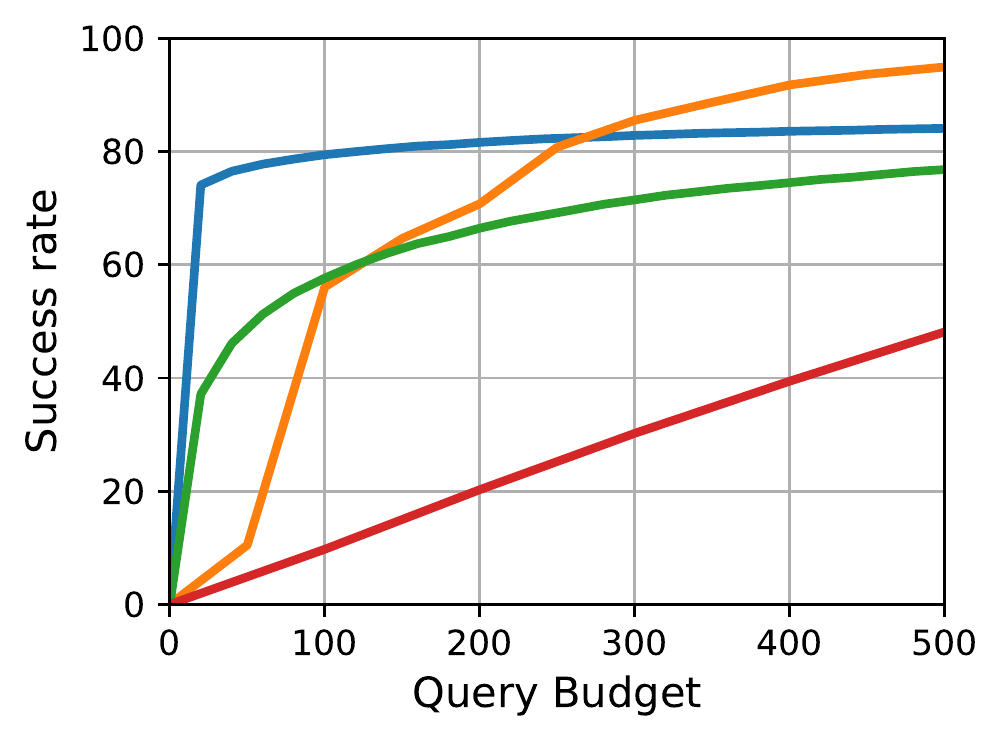}
   \caption{ {VGG16-bn}}
   \label{fig:vgg}
\end{subfigure}
\begin{subfigure}[b]{0.32\textwidth}
   \includegraphics[width=1\linewidth]{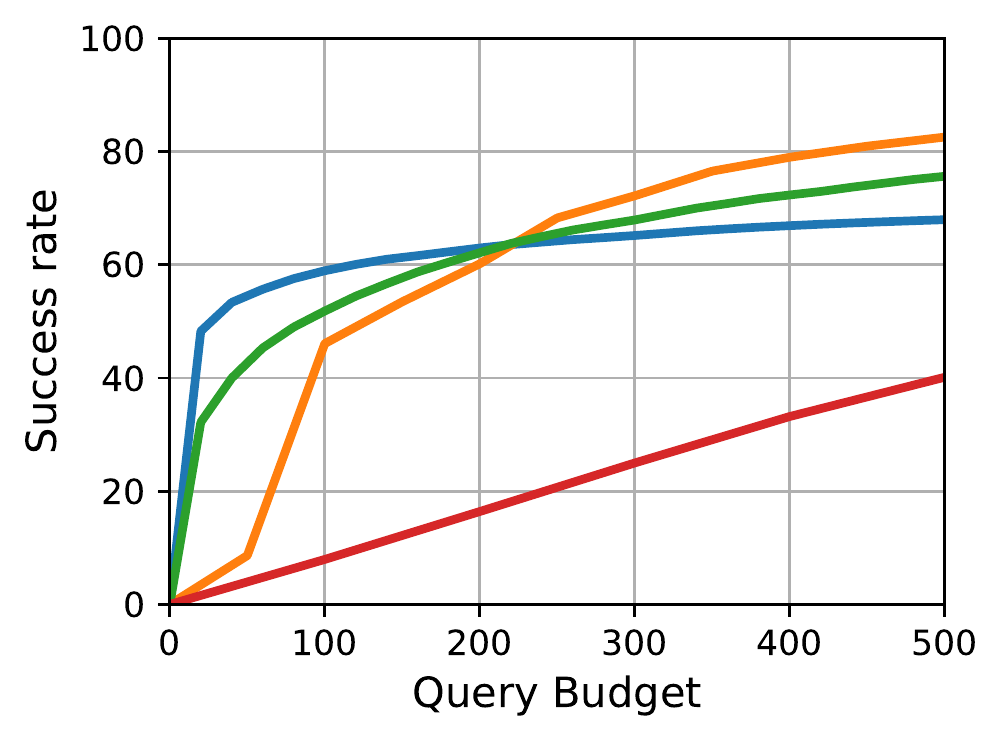}
   \caption{ {Inception-v3}}
   \label{fig:inception}
\end{subfigure}
\caption{Performance comparison for $\ell_\infty$ untargeted attacks on ImageNet classifiers.  { Bayes attack} consistently performs better for low query budgets $(\leq200)$. Note that for NES, model queries are performed in batches of 100 as specified in \citet{nes}.}
\label{fig:imagenet}
\end{figure*}

\begin{table*}[t]
\centering
\begin{tabular}{c c c c c} 
 \toprule
\multirow{2}{*}{ {Classifier}} & \multirow{2}{*}{ { Method}}&   {Success} &   {Average} &  {Median}\\
 & &  {Rate} &  {Query} &  {Query} \\
 \midrule
\multirow{4}{*}{  {ResNet50}} 
 &	 {NES}	            & $	15.20	\% $ & $	152	 $ & $	200	 $ \\
&	 {Bandits-TD}	    & $	56.59	\% $ & $	44	 $ & $	20	 $ \\
&	 {Parsimonious}	& $	72.26	\% $ & $	79	 $ & $	73	 $ \\
&	 { Bayes attack}	& $	\mbf{74.16}	\% $ & $	\mbf{17}	 $ & $	\mbf{6}	 $ \\
\midrule
\multirow{4}{*}{ {VGG16-bn}}
&	 {NES}	            & $	20.27	\% $ & $	152	 $ & $	200	 $ \\
&	 {Bandits-TD}	    & $	66.44	\% $ & $	40	 $ & $	16	 $ \\
&	 {Parsimonious}	& $	70.75	\% $ & $	80	 $ & $	73	 $ \\
&	 { Bayes attack}	& $	\mbf{81.60}	\% $ & $	\mbf{13}	 $ & $	\mbf{6}	 $ \\
  \midrule
  \multirow{4}{*}{ {Inception-v3}}
&	 {NES}	            & $	16.41	\% $ & $	152	 $ & $	200	 $ \\
&	 {Bandits-TD}	    & $	62.10	\% $ & $	45	 $ & $	20	 $ \\
&	 {Parsimonious}	& $	60.16	\% $ & $	84	 $ & $	74	 $ \\
&	 { Bayes attack}	& $	\mbf{62.95}	\% $ & $	\mbf{22}	 $ & $	\mbf{6}	 $ \\
 \bottomrule
 \end{tabular}
 \caption{Results for $\ell_\infty$ untargeted attacks on ImageNet classifiers with a query budget of $200$}
 \label{table:query_compare}
 \end{table*}

Figure \ref{fig:imagenet} compares the performance of the proposed method  {Bayes attack} against the set of baseline methods in terms of success rate at different query budgets. We can see that   {Bayes attack} consistently performs better than baseline methods for query budgets $<200$. Even for query budgets $>200$,  { Bayes attack} achieves better success rates than  {Bandits-TD} and  {NES} on ResNet50 and VGG16-bn. Finally, we note that for higher query budgets $(>1000)$, both {Parsimonious} and {Bandits-TD} method perform better than  {Bayes attack}.

To compare the success rate and average/median query, we select a point on the plots shown in Figure \ref{fig:imagenet}. Table \ref{table:query_compare} compares the performance of all the methods in terms of success rate, average and median query for a query budget of $200$. We can see that  { Bayes attack} achieves higher success rate with $80\%$ less average queries as compared to the next best attack method. 

\begin{figure}[h]
\centering
   \includegraphics[width=0.75\linewidth]{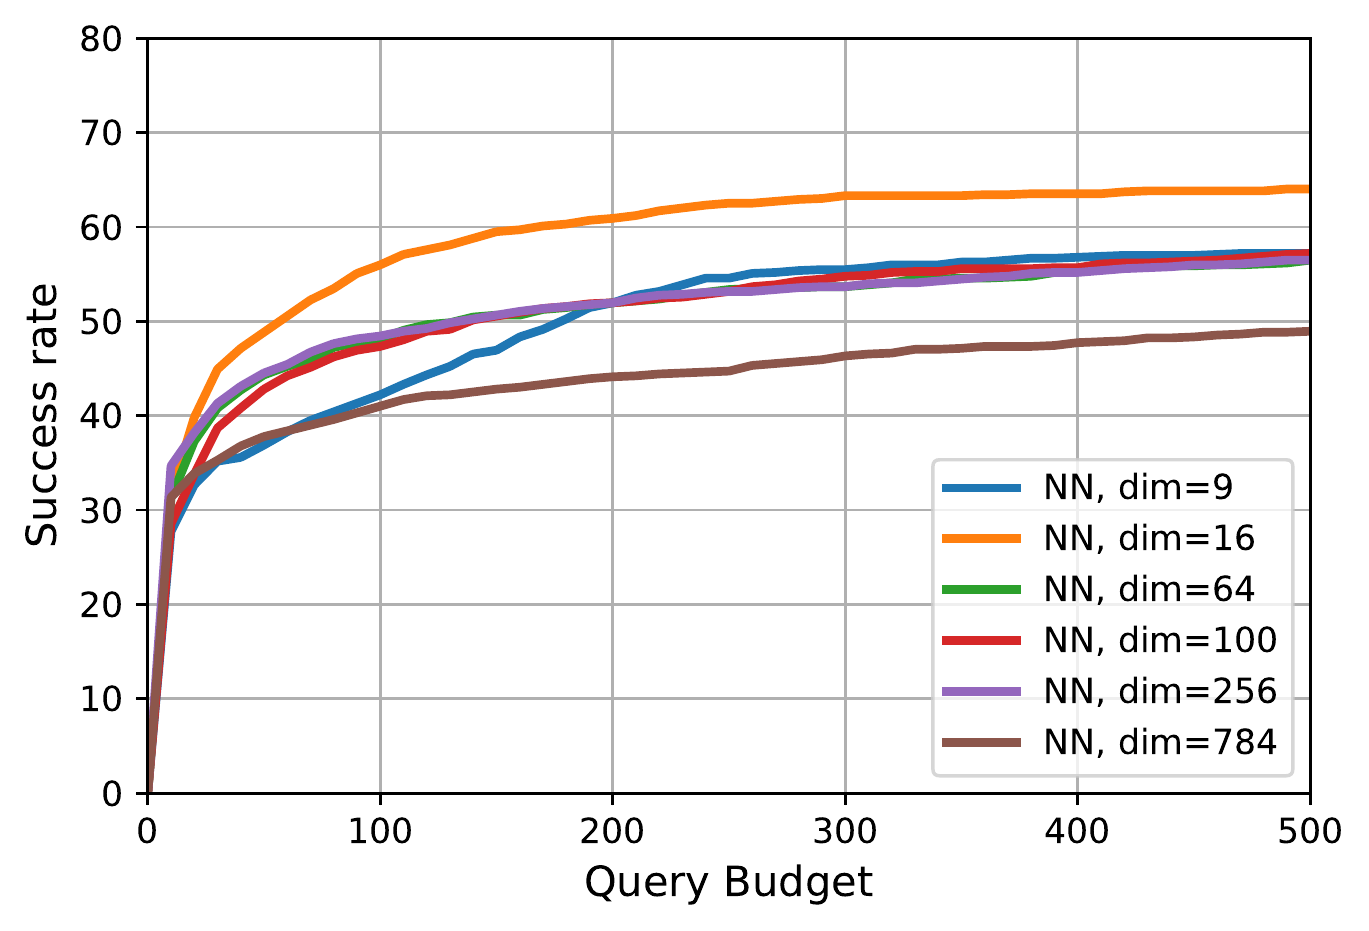}
   \caption{Performance comparison with different latent dimension.}
   \label{fig:dimension}
\end{figure}

\subsection{Latent Dimension Sensitivity Analysis}
We perform a sensitivity analysis on the latent dimension hyperparameter $d'$ used for running the Bayesian optimization on MNIST. We use the same network described in section 5 which achieves $99.5\%$ accuracy on MNIST test set. We conduct $\ell_\infty$ untargeted adversarial attacks with perturbation bound $\epsilon = 0.2$ on a randomly sampled $1000$ images from the test set. We vary the latent dimension over the range $d' \in \{9, 16, 64, 100, 256, 784\}$. Figure \ref{fig:dimension} shows the performance of nearest neighbor interpolation method for different latent dimension. We observe that lower latent dimensions achieve better success rates than the original input dimension $d'=784$ for MNIST. This could be because with increase in search dimension, Bayesian optimization needs more queries to find successful perturbation. 
We also note that for the case of latent dimension $d'=9$, {Bayes attack} achieves lower success rates which could mean that it is hard to find adversarial perturbations in such low dimension.

 \begin{figure}[h!]
\centering
   \includegraphics[width=0.6\linewidth]{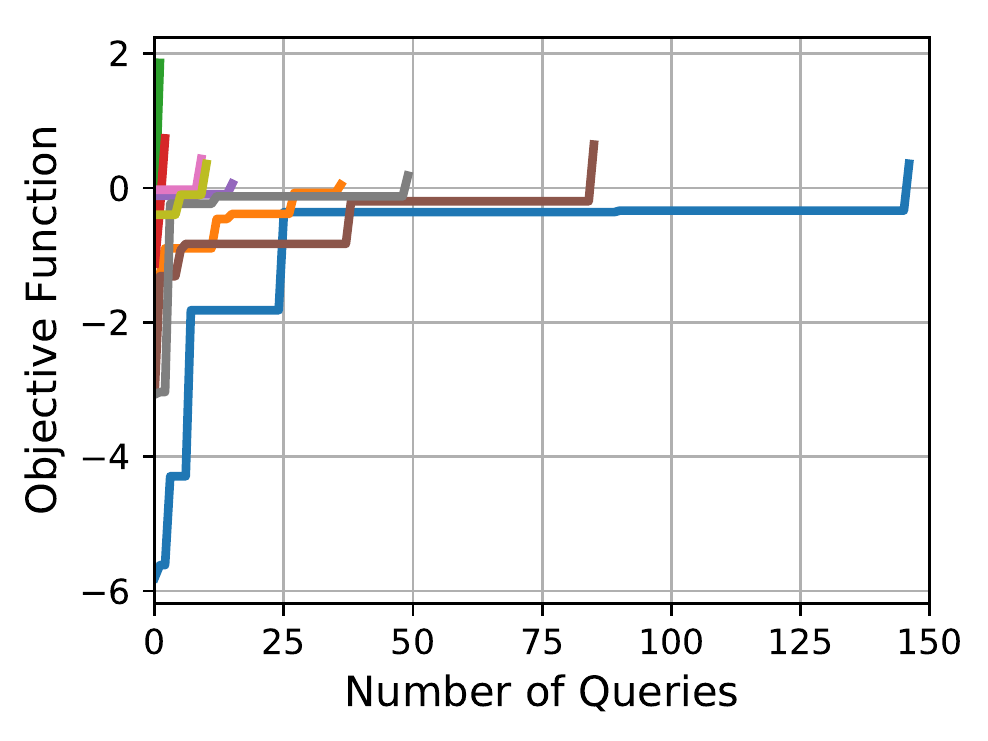}
   \caption{Convergence graphs on  {ResNet50} trained on ImageNet}
   \label{fig:resnet_convergence} 
\end{figure}

\begin{figure}[h!]
 \centering
   \includegraphics[width=\linewidth]{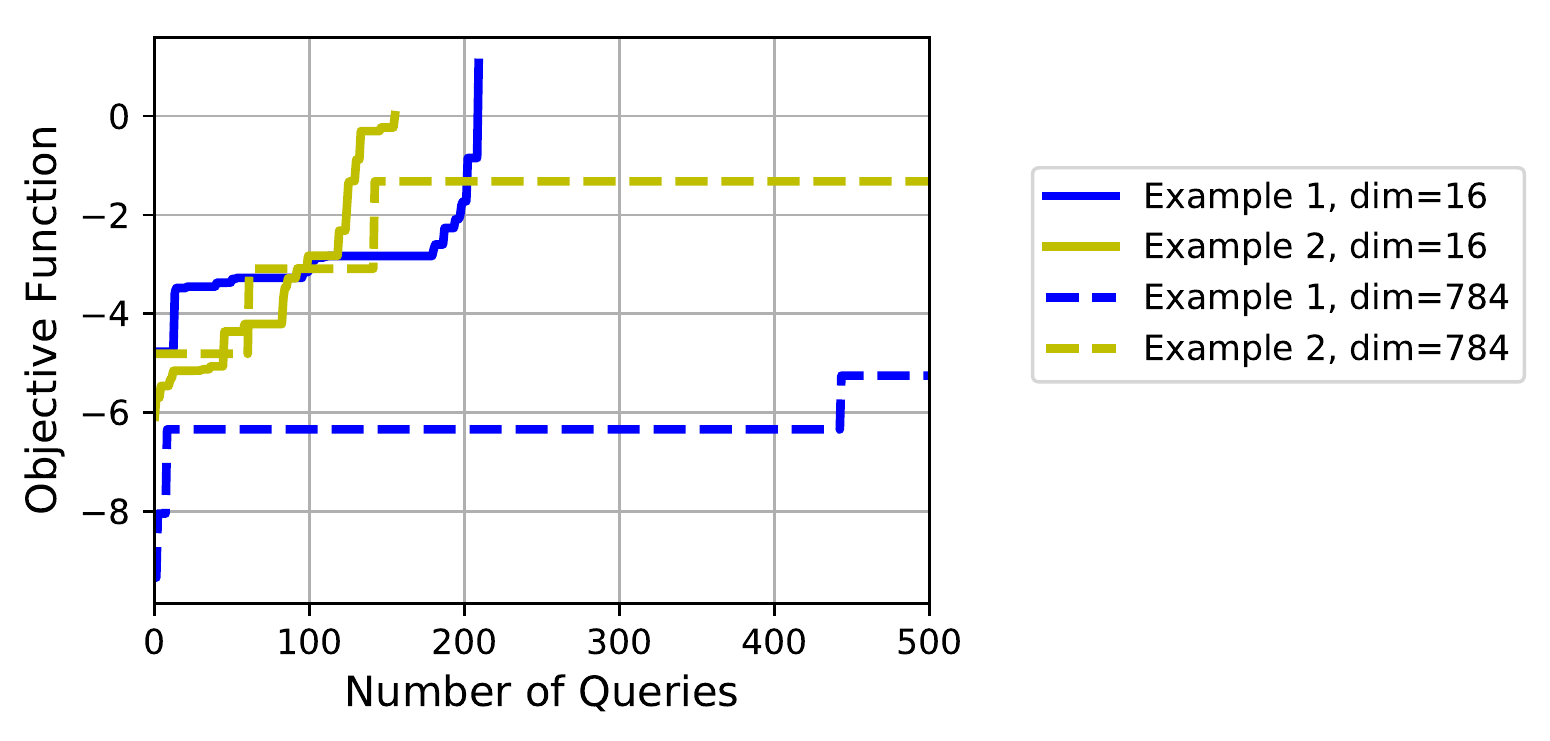}
   \caption{Convergence graphs on MNIST}
   \label{fig:mnist_convergence} 
\end{figure}

\subsection{Convergence of Bayes Attack}
\label{sec:convergence}
 In this section, we show the convergence of Bayesian Optimization (BO) in terms of objective value versus the number of queries. Note that we have framed our objective of finding adversarial perturbation to be a maximization problem and we stop the iteration loop of BO once the objective value reaches a positive value. A positive objective value corresponds to a successful adversarial perturbation as described in Section B. 
 
 Figure \ref{fig:resnet_convergence} shows the convergence of objective function in the  { Bayes attack} on  {ResNet50} trained on ImageNet. We run the BO in $972$ dimensions $(3\times18\times18)$ and upsample the perturbation to the original input dimension of $150,528  (3\times224\times224)$. The plot shows ten randomly chosen images from the validation set, with different colors representing different images.
 
We also show the convergence of the BO on MNIST by varying the latent dimension. Specifically, we compare the convergence with latent dimension $16 (4 \times 4)$ and the original input dimension $784 (28\times28)$. The plot is shown in Figure \ref{fig:mnist_convergence}. Each color represents a test image, while dashed lines and solid lines represent runs of BO using 16 and 784 dimensions, respectively. As we can see from the graph, BO in 784 dimensions does not converge to a successful attack (i.e., objective value $> 0$) in $500$ iterations on either of the images, while BO with $16$ dimensions on the same images finds the adversarial perturbation in less than $200$ iterations. This aligns with our observation that with increase in latent dimension, it becomes harder for BO to find successful perturbation and indeed it would require much more queries than running BO in lower dimensions.
